# Supplementary material for: Convex Combination Belief Propagation Algorithms
Source: arXiv:2105.12815 source file (2022-07-18)
Supplement: Supplementary file 1 [file appendix.tex]

\label{appendix}
\section{Message Passing in a Metric Space} % Main appendix title

Here is the appendix!
